# Supplementary material for: Nanoscale subsurface dynamics of solids upon high-intensity laser irradiation observed by femtosecond grazing-incidence x-ray scattering
Source: arXiv:2012.15076 ancillary file (2021-10-08)
Supplement: Supplementary file 1 [file Supplementary_Info_Nanoscale_subsurface_dynamics_Randolph_et_al_f.pdf]

## Supplementary Information for:

### Nanoscale subsurface dynamics of solids upon high-intensity laser irradiation observed by femtosecond grazing-incidence x-ray scattering

L. Randolph<sup>1</sup>, M. Banjafar<sup>2,3</sup>, T. R. Preston<sup>2</sup>, T. Yabuuchi<sup>4,5</sup>, M. Makita<sup>2</sup>, N. P. Dover<sup>6</sup>, Ch. Rödel<sup>7</sup>, S. Göde<sup>2</sup>, Y. Inubushi<sup>4,5</sup>, G. Jakob<sup>8</sup>, J. Kaa<sup>2</sup>, A. Kon<sup>6</sup>, J. K. Koga<sup>6</sup>, D. Ksenzov<sup>1</sup>, T. Matsuoka<sup>9,10</sup>, M. Nishiuchi<sup>6</sup>, M. Paulus<sup>11</sup>, F. Schon<sup>1</sup>, K. Sueda<sup>5</sup>, Y. Sentoku<sup>10,12</sup>, T. Togashi<sup>4,5</sup>, M. Vafae-Khanjani<sup>8</sup>, M. Bussmann<sup>13</sup>, T. E. Cowan<sup>3,13</sup>, M. Kläui<sup>8</sup>, C. Fortmann-Grote<sup>2</sup>, A. P. Mancuso<sup>2,14</sup>, T. Kluge<sup>13</sup>, C. Gutt<sup>1</sup> and M. Nakatsutsumi<sup>2,9</sup>

<sup>1</sup> *Department Physik, Universität Siegen, Walter-Flex-Str. 3, 57072 Siegen, Germany*

<sup>2</sup> *European XFEL, Holzkoppel 4, 22869 Schenefeld, Germany*

<sup>3</sup> *Technical University Dresden, 01069 Dresden, Germany*

<sup>4</sup> *Japan Synchrotron Radiation Research Institute (JASRI), Sayo, Hyogo 679-5198, Japan*

<sup>5</sup> *RIKEN SPring-8 Center, Sayo, Hyogo 679-5148, Japan*

<sup>6</sup> *QST-Kansai, KPSI, 8-1-7 Umemi-dai, Kizugawa-city, Kyoto, 619-0215, Japan*

<sup>7</sup> *Technical University Darmstadt, Schlossgartenstraße 9, 64289 Darmstadt, Germany*

<sup>8</sup> *Universität Mainz, Staudinger Weg 7, 55128 Mainz, Germany*

<sup>9</sup> *Open and Transdisciplinary Research Institute, Osaka University, Suita, Osaka 565-0087, Japan*

<sup>10</sup> *Graduate School of Engineering, Osaka University, Suita, Osaka 565-0087, Japan*

<sup>10</sup> *Technische Universität Dortmund, August-Schmidt-Straße 1, 44227, Germany*

<sup>11</sup> *Technical University Dortmund, Otto-Hahn Straße 4, 44227 Dortmund, Germany*

<sup>12</sup> *Institute of Laser Engineering, Osaka University, Suita, Osaka 565-0871, Japan*

<sup>13</sup> *Helmholtz-Zentrum Dresden-Rossendorf, Bautzner Landstraße 400, 01328, Dresden, Germany*

<sup>14</sup> *Department of Chemistry and Physics, La Trobe Institute for Molecular Science, La Trobe University, Melbourne, Victoria 3086, Australia*

#### S.1 GISAXS data set

Fig S1 shows the density profiles for all measured time delays and Fig. S2a and S2b present the full GISAXS dataset with lineouts of the in-plane scattering and the corresponding real-space density profiles. From top to bottom in S2 a,b) we observe systematic changes in the scattering signal with the pump-probe delay. At small delay (up to 2.5 ps) there is a clear reduction in the number of Kiessig fringes in the scattering signal, indicating a decrease in the number of layers. At later times (> 3.0 ps), additionally, the central Bragg peak starts to vanish, which indicates a disappearing of the double layer periodicity. At 6.0 ps, the Bragg peak is almost completely washed out.

Fig. S3 shows the corresponding out-of-plane scattering signals that are used together with the in-plane scattering to retrieve the real-space density profiles shown in Fig S2a and S2b. Details of the fitting procedures of the out-of-plane signal is discussed in section S.4.

## S.2 X-ray reflectivity (XRR) measurement for ML characterization

The x-ray reflectivity (XRR) measurements were performed at the beamline BL9 of the synchrotron radiation source DELTA, Dortmund as shown in Fig. S4. The photon energy was 13 keV ( $\lambda = 0.954 \text{ \AA}$ ). The beam dimensions were  $0.1 \times 1.5 \text{ mm}^2$  (vertical x horizontal). A PILATUS100k (Dectris, Switzerland) x-ray detector was used for photon detection. Refinement of the data yielded the electron density profile shown in Fig. S4b. The inset in Fig. S4a displays the relevant Q-range for the GISAXS setup used at our SACLA experiment representing the characteristic Bragg peak at  $Q_z = 1.33 \text{ nm}^{-1}$  and the four Kiessig fringes on the left.

## S.3 Background modeling in GISAXS data

Fig. S5 shows the GISAXS signal from a typical preshot (x-ray only). The specular peak located at  $Q_0 = 0.99 \text{ nm}^{-1}$  is orders of magnitude more intense than the remaining GISAXS signal and is blocked by a beamstop in the experiment. The tails of the parasitic scattering from the beamstop have been modeled via  $(Q_z - Q_0)^{-x}$  with  $x$  denoting an adjustable parameter with slightly different magnitudes for  $Q_z$  values above or below the specular position (see Fig. S5). Taking this background into account, the solid line in Fig. S5 represents the predicted scattering signal from the density profile shown in Fig. 4b.

## S.4 Model refinement using simultaneous in-plane and out-of-plane scattering signals

A simultaneous data refinement of in-plane and out-of-plane scattering signals appeared crucial to mitigate problems of having non-unique solutions when retrieving the density profile from the given scattering data, which are exacerbated by the limited  $Q_z$  range available in the experimental setup. The in-plane signal represents an average of a region of 30 pixels centered around the position of  $Q_y = 0 \text{ nm}^{-1}$ . The out-of-plane signal is an average of the scattering signal within an interval  $Q_y = 0.15 \text{ nm}^{-1}$  to  $0.5 \text{ nm}^{-1}$ .

Both in-plane and out-of-plane signals at a delay of 2 ps are displayed in Fig. S6 as a function of the corresponding vertical wave vector transfer  $Q_z$ . The out-of-plane signal not only depends on the density profile but also on roughness correlations between the layers. These correlations are modeled in the program BornAgain with the following statistical description of the height-height correlation function for the  $j^{\text{th}}$  interface with height contour  $U_j(x, y)$ ,

$$\langle U_j(x, y)U_j(x', y') \rangle = \sigma^2 \exp \left[ - \left( \frac{\tau}{\xi_{Lj}} \right)^{2h} \right],$$

where

$$\tau = \sqrt{(x - x')^2 + (y - y')^2}.$$

We observed that the  $Q_z$ -dependence of the off-specular signal is not very sensitive to the absolute value of the lateral correlation lengths  $\xi_L$ , although it is quite sensitive to *differences* in the correlation lengths between different layers in the following way: the correlation lengths  $\xi_L \geq 30 \text{ nm}$  switches the contribution from the corresponding layer to the out-of-plane signal "on" while a small value of  $\xi_L = 1 \text{ nm}$  switches the contribution to the signal "off". Upon pumping we find that the in-plane correlation lengths decrease starting from the top layers. In contrast, the vertical correlation length  $\xi_{\perp}$  needs to be kept at the value on the order of the ML thickness in order to make the scattering signal visible, to reproduce the experimental result.

We illustrate this in Figures S6a and S7a by displaying two different density profiles (right) and corresponding in-plane scattering signal (left) for  $t = 2$  and  $3.5$  ps, respectively. While both modeled signals look similar to a certain extent we find a clear difference in the corresponding  $\chi^2$  values favoring the blue density profile. Further evidence for this can be obtained by inspecting the corresponding out-of-plane scattering signal.

Fig. S6b and S7b display the out-of-plane scattering signal for both density profiles with various lateral correlation lengths  $\xi_L$  from top to bottom (layer 1 is the topmost layer and layer 14 the layer closest to the substrate) as summarized below:

| Figure S6b | $\xi_L = 1$ nm | $\xi_L = 30$ nm   | $\chi^2$ blue profile | $\chi^2$ red profile |
|------------|----------------|-------------------|-----------------------|----------------------|
| 1          | -              | layer 1-14        | 8928                  | 5268                 |
| <b>2</b>   | <b>layer 1</b> | <b>layer 2-14</b> | <b>1667</b>           | <b>4810</b>          |
| 3          | layer 1-6      | layer 7-14        | 2948                  | 4291                 |
| 4          | layer 1-12     | layer 13-14       | 2209                  | 3583                 |

| Figure S7b | $\xi_L = 1$ nm    | $\xi_L = 30$ nm    | $\chi^2$ blue profile | $\chi^2$ red profile |
|------------|-------------------|--------------------|-----------------------|----------------------|
| 1          | -                 | layer 1-14         | 3013                  | 3298                 |
| 2          | layer 1-3         | layer 4-14         | 11180                 | 3249                 |
| <b>3</b>   | <b>layer 1-10</b> | <b>layer 11-14</b> | <b>1114</b>           | <b>3474</b>          |
| 4          | layer 1-12        | layer 13-14        | 1243                  | 3133                 |

As shown in Fig. S6b and Fig. S7b and also in the plot of  $\chi^2$  the blue density profile fits the out-of-plane signal significantly better than the red density profile. This is also apparent from an inspection of the difference trace (light blue and red lines). Furthermore, to demonstrate the sensitivity of the out-of-plane scattering signal for actual electron density profile, we systematically reduced the density profile at  $t = 2$  ps layer by layer starting from the top (Fig. S8). This shows that the density profile has a pronounced influence on the out-of-plane scattering signal as well.

To conclude, a simultaneous inspection of in-plane and out-of-the plane scattering components helps considerably to narrow down the search for density profiles. However, an extension of the available  $Q_z$ -space would be beneficial to provide further constraint. We note that the refinement procedure applied here does not exclude the existence of other density profiles providing different local minima in parameter space.

## S.5 Laser intensity profile, effect of spatial intensity variation

Due to the grazing incidence, the x-ray footprint on sample has an ellipsoidal profile elongated in one direction,  $4 \mu\text{m} \times \sim 360 \mu\text{m}$ . In order to match to the x-ray footprint, the laser was defocused from the best focus position. Figure S9 shows the laser profile on the sample and its lineout. The averaged laser intensity over the area probed by the x-ray was  $3.8 \times 10^{14} \text{ W.cm}^{-2}$ . With  $17^\circ$  angle of incidence, this intensity is decreased by a factor of  $\cos(17^\circ)^{-1}$ , i.e.,  $3.6 \times 10^{14} \text{ W.cm}^{-2}$ . The local intensity varies between  $2 - 5 \times 10^{14} \text{ W.cm}^{-2}$ . Figure S10 shows the electron temperature taken at 40 fs after the laser temporal peak and the velocity of the heat front as a function of the laser intensity extracted from the Multi-fs hydrodynamic simulation. Although the peak temperature increases linearly with laser intensity (blue circles), the velocity of the heat front (red diamonds) depends weakly with the intensity. This is because the heat conductivity is a function of the collision frequency, the value of which does not change significantly around the Fermi temperature. The velocity is slightly decreased when it goes below the

Fermi temperature (i.e.,  $2$  and  $3 \times 10^{14} \text{ W.cm}^{-2}$ ), as the collision frequency reaches its peak value around the Fermi temperature.

The average laser pulse energy on the sample was  $53 \text{ mJ}$  ( $67 \text{ mJ}$  before the pulse compressor). Shot-to-shot energy fluctuation was  $5.7 \text{ mJ}$  in standard deviation. The on-sample laser pulse energy for each shot used in our analysis is summarized below.

| Delay (ps) | Run number | Laser energy on sample (mJ) |
|------------|------------|-----------------------------|
| 0.5        | 49130      | 54.4                        |
| 1.0        | 49147      | 52                          |
| 1.5        | 49150      | 51.2                        |
| 2.0        | 49162      | 50.8                        |
| 2.5        | 49153      | 57.6                        |
| 3.0        | 49138      | 64.4                        |
| 3.5        | 49159      | 56                          |
| 4.0        | 49168      | 56.3                        |
| 5.0        | 49142      | 57.6                        |
| 6.0        | 49186      | 44.8                        |

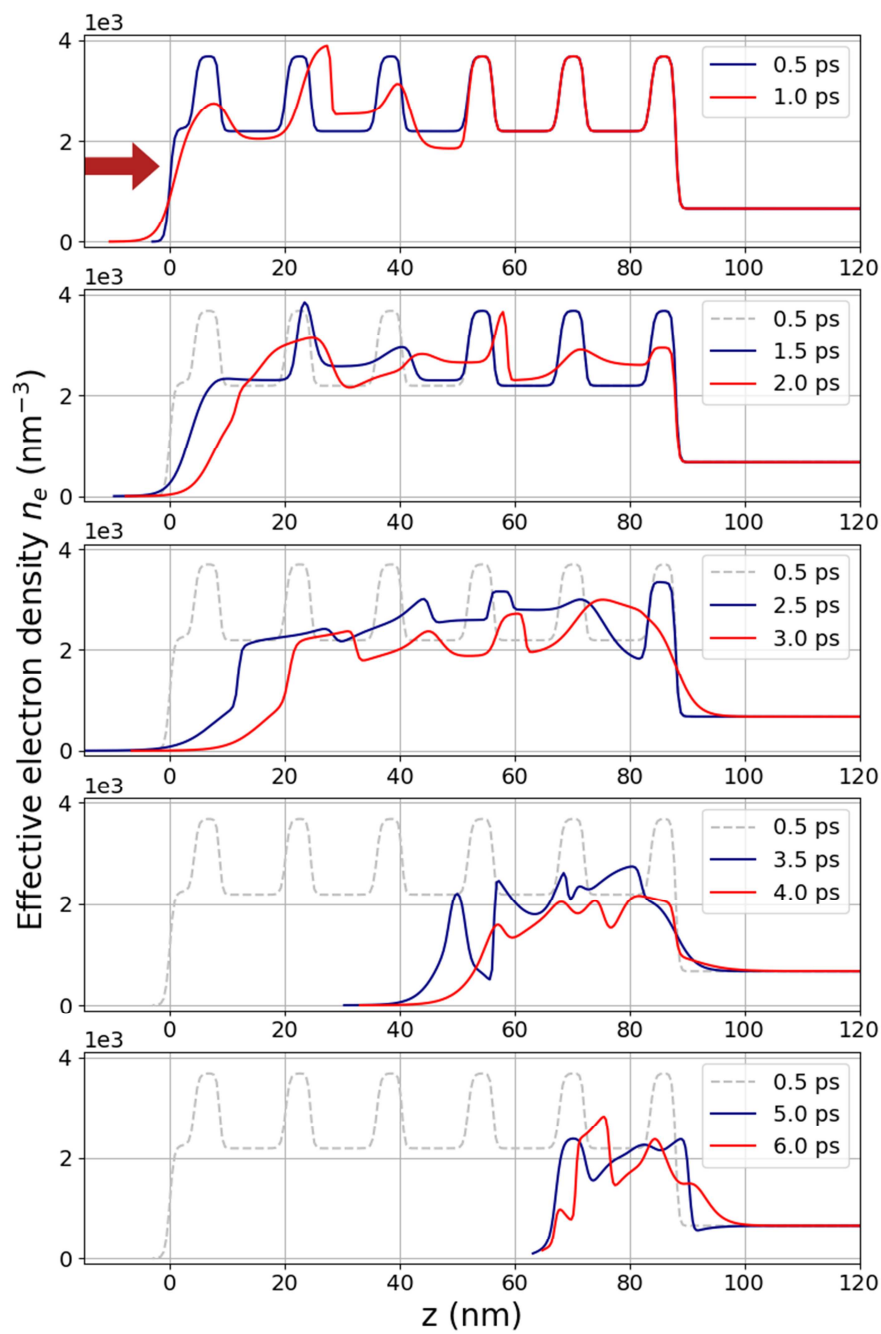

**Fig. S1.** Summary of electron density profiles extracted from the GISAXS data for all time delays from 0.5 ps up to 6.0 ps. The laser comes from the left (red arrow).

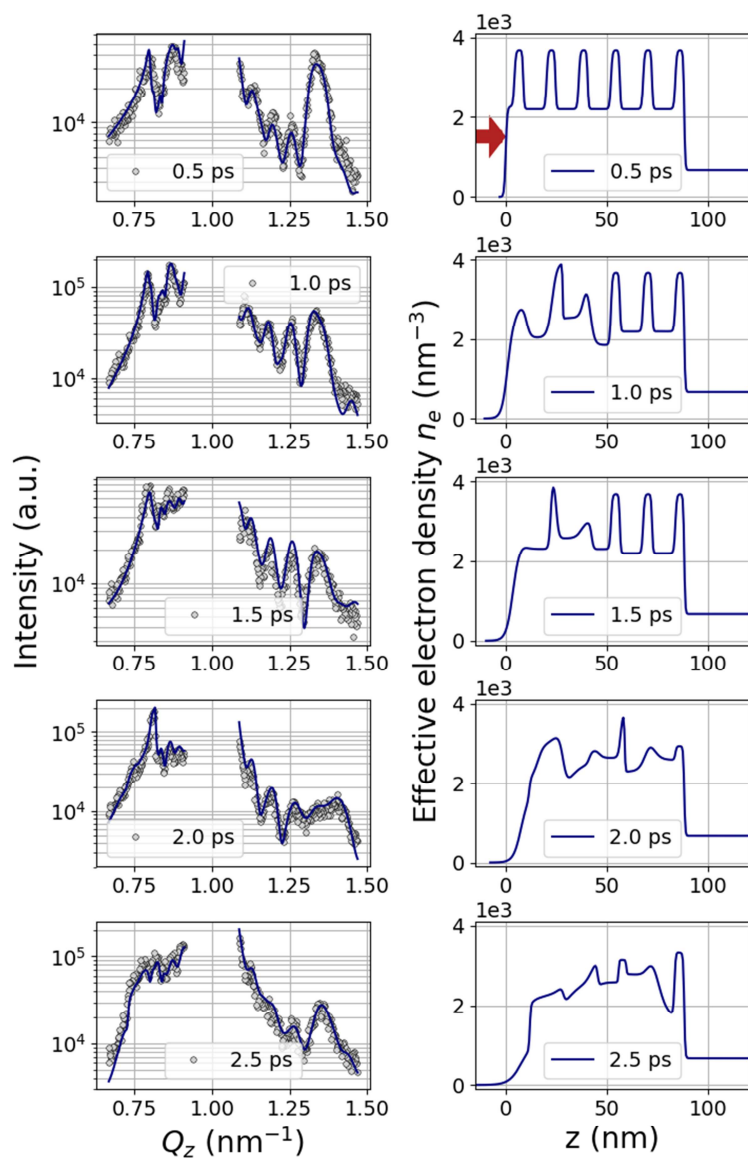

**Fig. S2a.** (left) In-plane scattering signal with refinements (blue solid lines) and (right) corresponding density profiles for time delays between 0.5 ps and 2.5 ps. The laser comes from the left (red arrow).

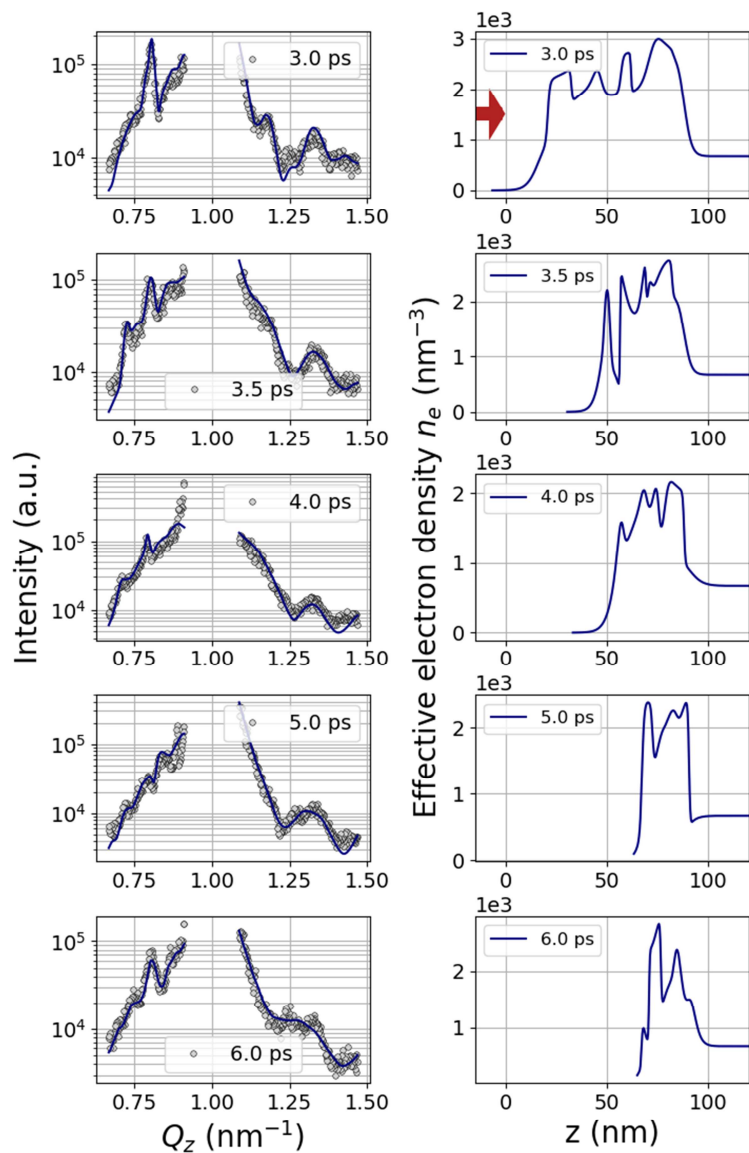

**Fig. S2b.** (left) In-plane signal with refinements (solid lines) and (right) corresponding density profiles for time delays between 3.0 ps and 6.0 ps. The laser comes from the left (red arrow).

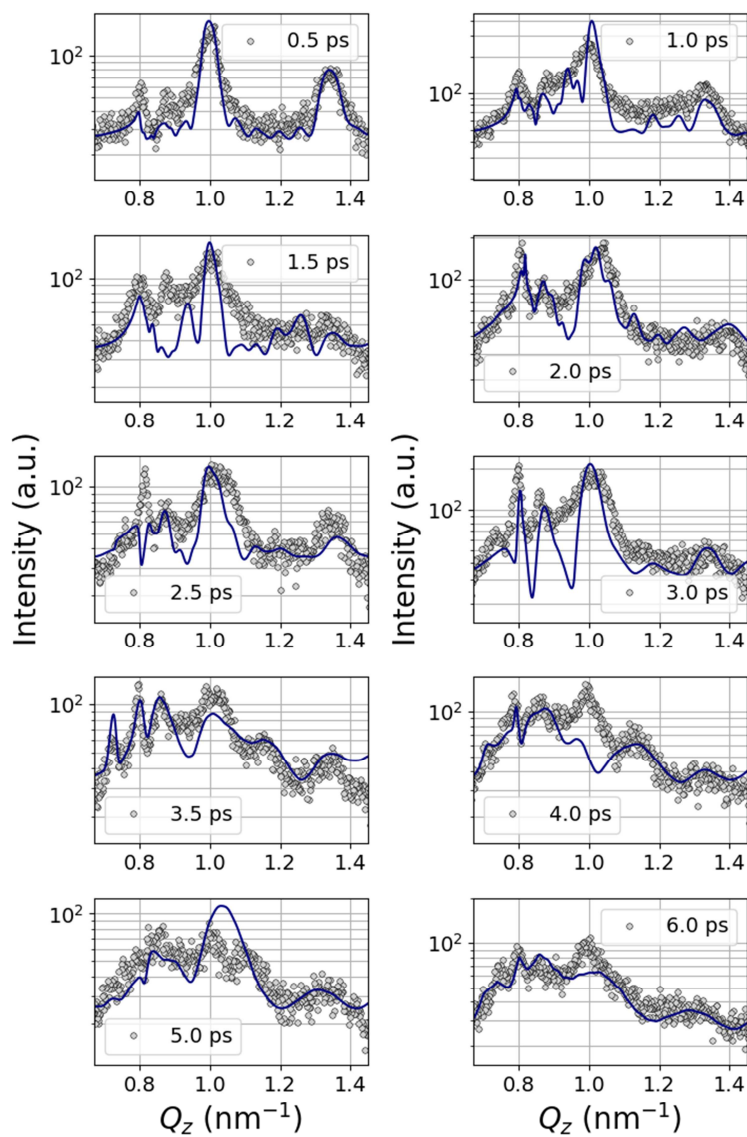

Fig. S3. Out-of-plane scattering signal with refinement (solid lines) using the same density profiles as for the in-plane scattering signal (see Fig. S2a and S2b) and adjusting the lateral correlation length  $\xi_L$ .

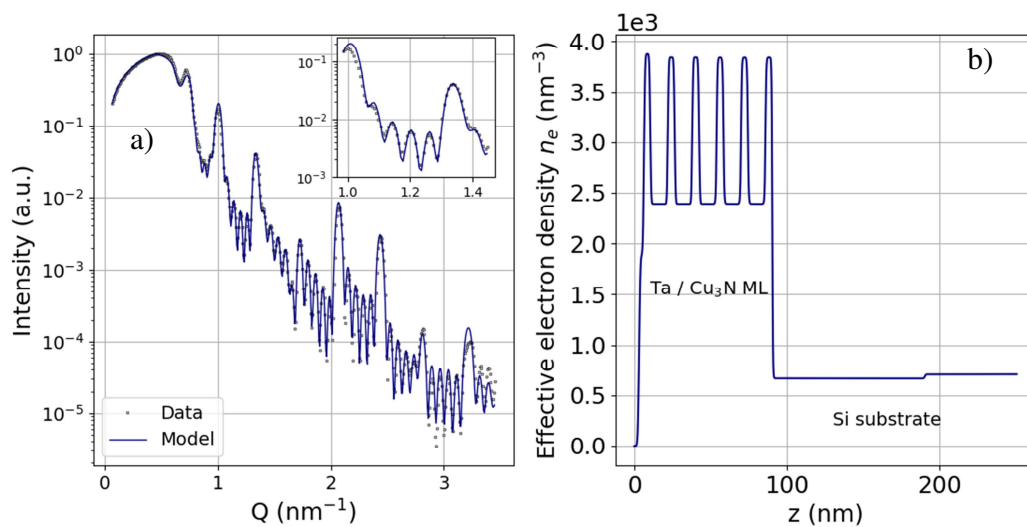

**Fig. S4.** *a)* X-ray reflectivity (XRR) curve of the ML recorded with a photon energy of 13 keV at a synchrotron. The inset displays the relevant  $Q$ -range covered in our GISAXS experiment with a central Bragg peak located at  $Q = 1.35 \text{ nm}^{-1}$  and four characteristic Kiessig fringes. *b)* Effective electron density profile deduced from modeling the XRR data (solid lines in XRR curve).

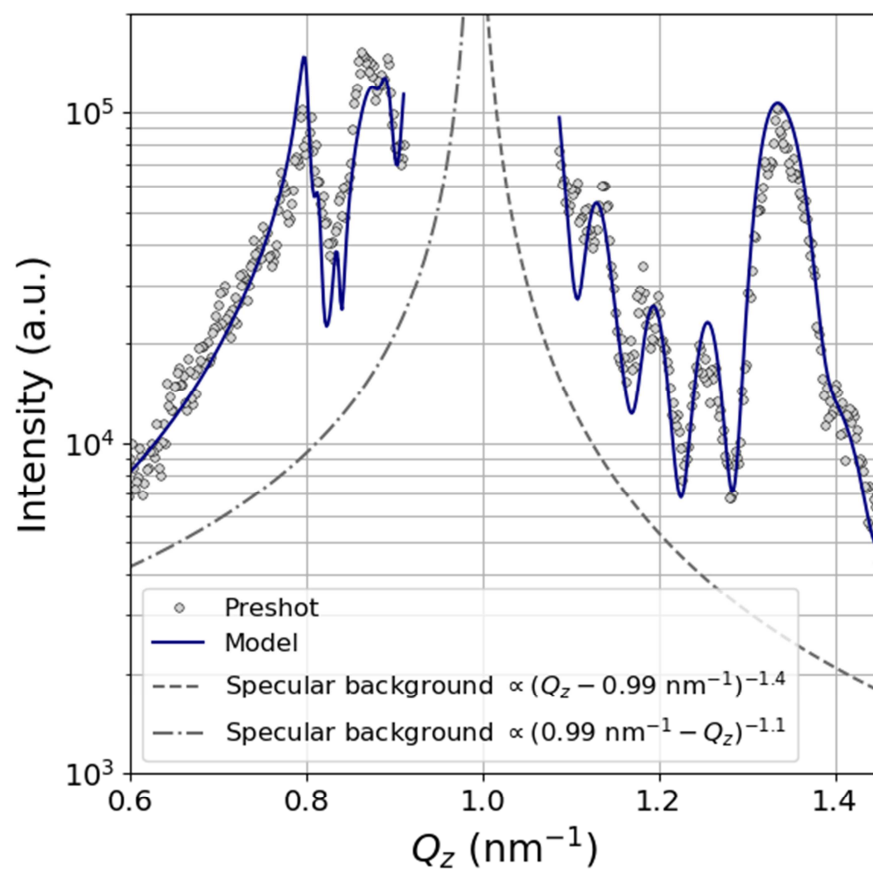

**Fig. S 5.** Grey points: GISAXS data from a preshot. The grey dashed line and dash-dotted line represent the model accounting for parasitic scattering tails from the beamstop used to block the highly intense specular signal at  $0.99 \text{ nm}^{-1}$ . The blue solid line shows the model based on the density profile from Fig. S4 including the background.

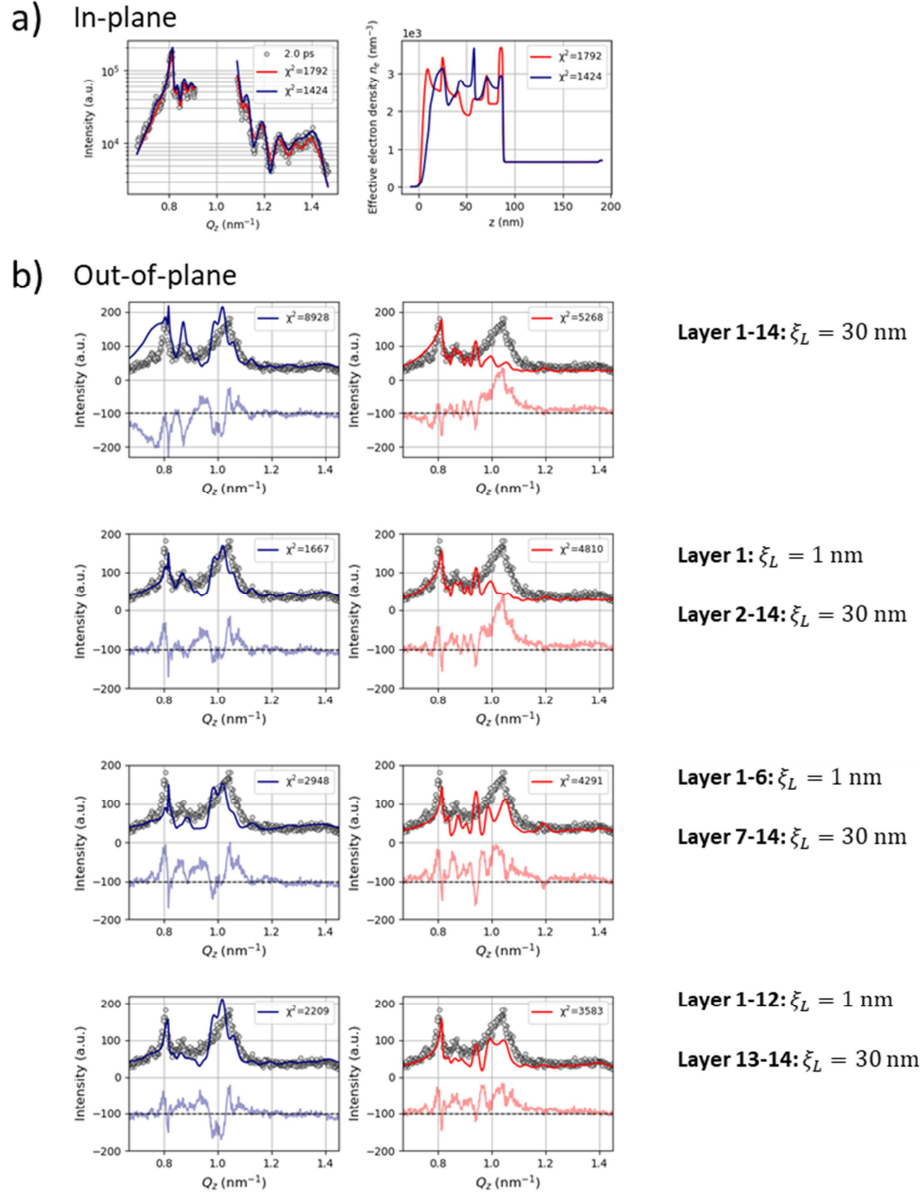

**Fig. S 6. a)** In-plane scattering signal at the delay 2 ps with refinement using two different density profiles as shown on the right hand side. **b)** Corresponding out-of-plane scattering signal and refinement by using a different number of laterally correlated layers applied for the blue (left) and red (right) density profile (for details see text). The corresponding values of  $\chi^2$  are also displayed.

a) In-plane

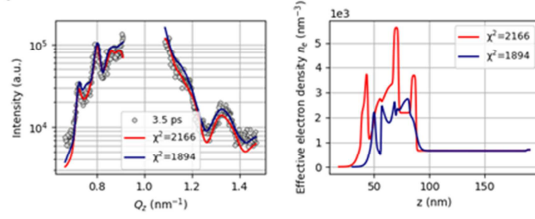

b) Out-of-plane

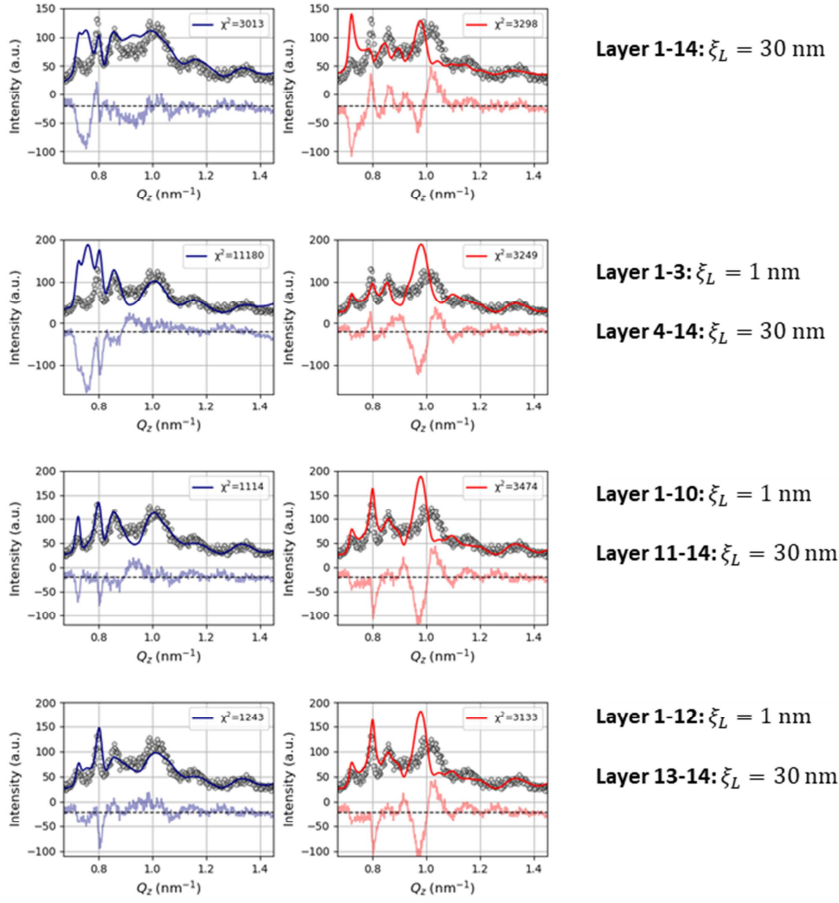

**Fig. S 7. a)** In-plane scattering signal at the delay 3.5 ps with refinement using two different density profiles as shown on the right hand side. **b)** Corresponding out-of-plane scattering signal and refinement by using a different number of laterally correlated layers applied for the blue(left) and red (right) density profile (for details see text). The corresponding values of  $\chi^2$  are also displayed.

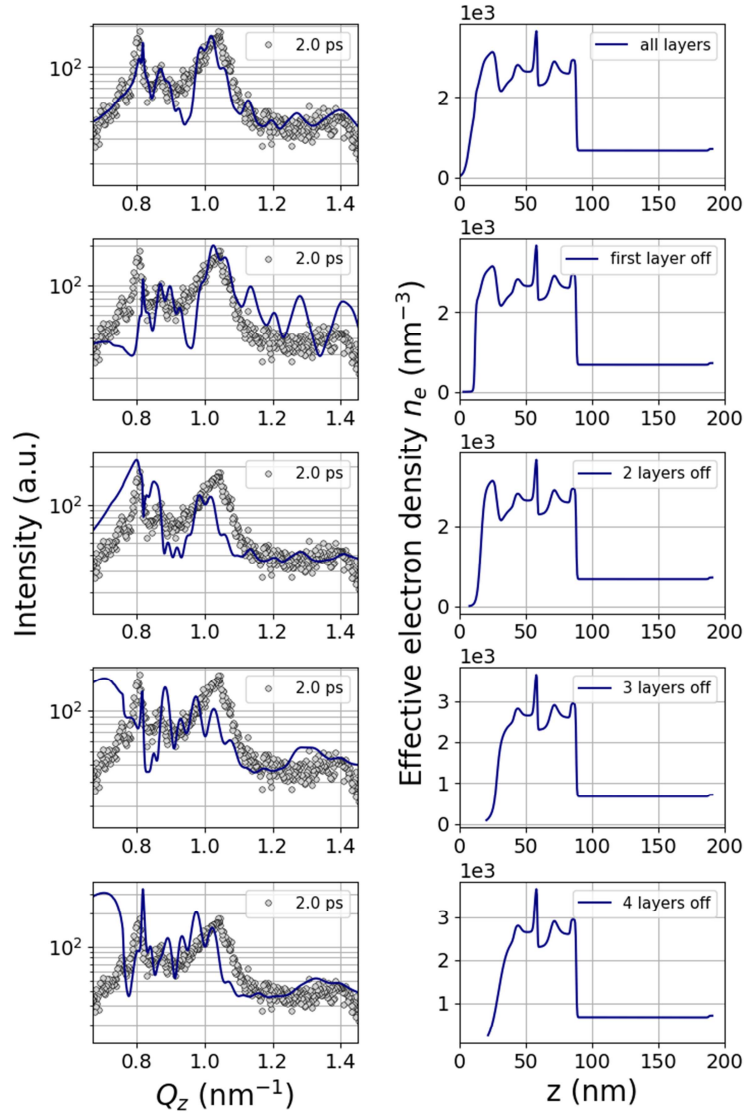

**Fig. S8.** **(left)** Out-plane scattering signal at the delay of 2.0 ps. **(right)** Density profiles with consecutive layers removed from the top to illustrate the influence of the density profile onto the out-of-plane scattering signal.

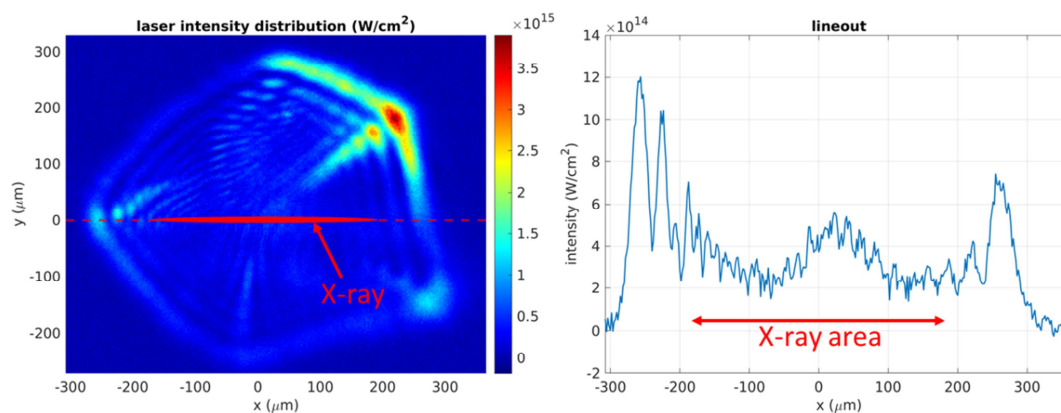

**Fig. S9.** Laser profile used for the experiment. **(left)** Laser intensity profile irradiated on the sample. The red horizontal area corresponds to the x-ray area. **(right)** Corresponding lineout of the intensity profile. The averaged intensity where probed by the x-ray is  $3.8 \times 10^{14} \text{ W.cm}^{-2}$  which is decreased to  $3.6 \times 10^{14} \text{ W.cm}^{-2}$  by taking into account the incident angle of  $17^\circ$  from the sample normal.

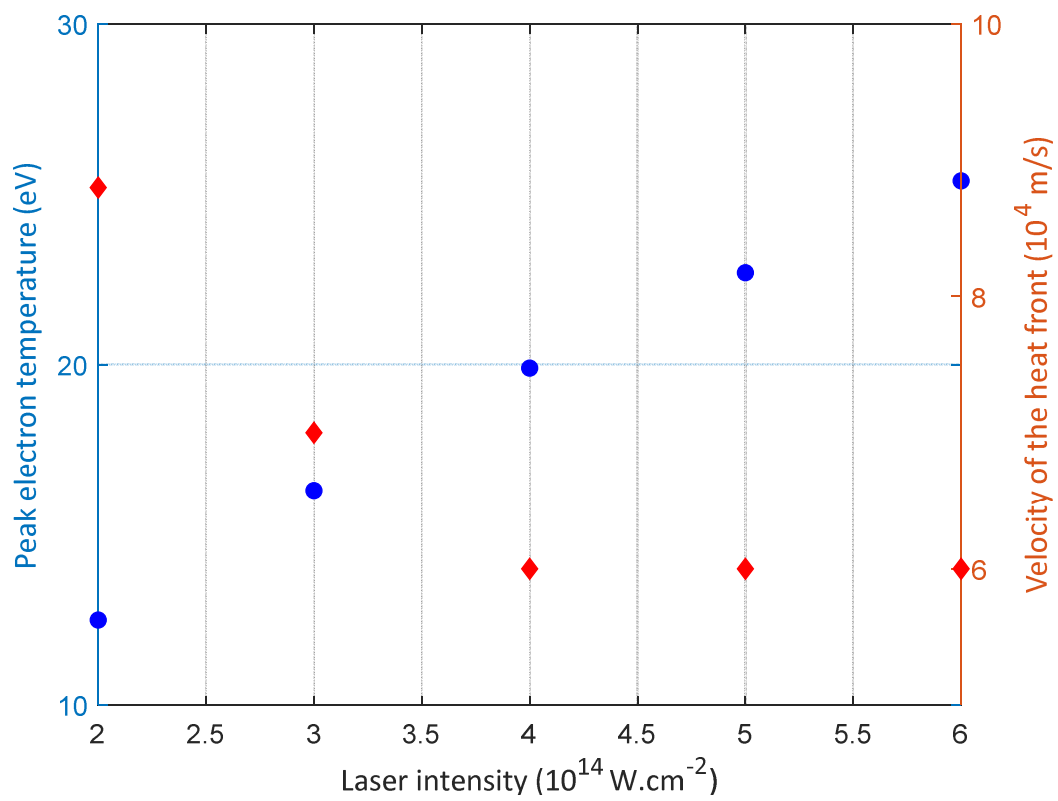

**Fig. S10.** The electron temperature taken at 40 fs after the intensity peak and the velocity of the heat front (before it reached the substrate) extracted from Multi-fs hydrodynamic simulation. The heat front position is defined as the position where the temperature is decreased by  $1/e$ . As shown in the Fig. 4 in the main text, this velocity is almost constant with time.
